# Supplementary material for: A Comprehensive Survey of Multilingual Neural Machine Translation
Source: arXiv:2001.01115 source file (2020-01-07)
Supplement: Supplementary file 1 [file supplementary.tex]

% \documentclass{article}
% \usepackage[utf8]{inputenc}
% \usepackage{multicol}
% \usepackage{multirow} 

% \title{A Survey of Multilingual Neural Machine Translation - Supplementary Material}
% \author{}
% \date{}

% \begin{document}

% \maketitle

\begin{table}[]
    \centering
    \begin{tabular}{|l|l|}
         \hline
         \multicolumn{2}{|c|}{\textbf{Multiway}}  \\
         \hline
         \multicolumn{2}{|l|}{\textbf{Prototypical Approaches}} \\ \hline 
         Complete Sharing & \cite{ha16}, \cite{johnson17},   \cite{aharoni19}, \cite{sachan18} \\       \hline
         Minimal  Sharing & \\         \hline
         \multicolumn{2}{|l|}{\textbf{Controlling Sharing}} \\ \hline
         General & \\         \hline
         Dynamic Parameter Generation & \\         \hline
         Universal Encoder Representation & \\ \hline 
         Multiple Target Languages & \\         \hline
         \multicolumn{2}{|l|}{\textbf{Training Protocols}} \\ \hline
         Joint Training & \\         \hline
         Knowledge Distillation & \\        
         \hline
         \multicolumn{2}{|c|}{\textbf{Low or Zero-Resource}}  \\
         \hline 
         \multicolumn{2}{|l|}{\textbf{Transfer Learning}}\\ \hline 
         \multicolumn{2}{|l|}{\textbf{Pivot}} \\ \hline
         \multicolumn{2}{|l|}{\textbf{Zeroshot}} \\ \hline 
         
         \hline
         \multicolumn{2}{|c|}{\textbf{Multi-source}}  \\
         \hline
         Multi-source available & \\         \hline
         Missing source sentences & \\         \hline
         Post-editing & \\
         \hline
    \end{tabular}
    \caption{Caption}
    \label{tab:Related Works}
\end{table}

% \bibliography{acl2019_mnmt}
% \bibliographystyle{acl_natbib}

% \end{document}
